# Supplementary material for: Invisible and Semi-invisible Decays of Bottom Baryons
Source: arXiv:2404.04337 source file (2024-08-19)
Supplement: Supplementary file 1 [file 8-Appendix.tex]

\appendix

%%%%%%%%%%%%%%%%%%%%%%%%%%%%%%%%%%%%%%%%%%%%%%%%%%%%%%%%%%%%%

\section{The coupling constant of $\Lambda_Q$ baryon in QCD sum rules}{\label{Appen-QCD-input}}
When evaluating the correlation function \eqref{eq_correlator} at leading order of $\alpha_s$ and the vaccum condensates up to dimension $d=6$, the corresponding diagrams are illustrated in FIG.\ref{Fig:Baryon_correlator-total}.
\input{Feynman-diagram/total_per_and_non-per}
The analytical results for Eq. \eqref{eq:final-result} are given by,
\begin{equation}{\label{eq:OPE_result}}
                 \begin{aligned}
             % \mathcal{J}_{\Lambda_Q} &= \epsilon^{ijk} \left[  u_i^T C \gamma_5 d_j \right] P_R Q_k, \\
            \mathbf{Im}\Pi^{(pert)}_{\Lambda_Q, 0}(s) 
           &= \frac{m_Q^4}{2^{9}\pi^3} \left(   
           \frac{1}{x^2} - \frac{8}{x} +8x -  x^2
           -12ln(x)
           \right), \\
            \mathbf{Im} \Pi^{(\left< \bar{q}q \right>)}_{\Lambda_Q, 0} (s) 
          &=- 
          \frac{m_q \left<\bar{q}q\right>}{2^4\pi}   (1-x^2),
          \\
            \mathbf{Im} \Pi^{(\left< GG\right>)}_{\Lambda_Q, 0} (s)
         &=  \frac{\left<g^2_s G^2\right>}{3 \cdot 2^{10} \pi^3} (1 + 4x-5x^2),
          \\
         \Pi^{(\left<\bar{q} G q \right>)}_{\Lambda_Q, 0}(s) 
          &=  \frac{7 m_q\left< \bar{q}Gq \right>}{3 \cdot 2^5 \pi^2 (m_Q^2- s)}, \\
             \Pi^{(\left< \bar{q}q \right>^2)}_{\Lambda_Q, 0} (s)
                 &=
                \frac{{\left< \bar{q}q \right>^2}}{6(m_Q^2-s)},
                 \end{aligned} 
           \end{equation}
where $x= \frac{m_Q^2}{s}$. 
To determine the numerical values of coupling constant $\lambda_{\Lambda_b}$, the input parameters are listed as follow: 
$m_b = 4.60 \pm 0.10 \ \text{GeV}$, 
$m_c = 1.35 \pm 0.10 \ \text{GeV}$,
$m_s = 0.12  \pm 0.01\ \text{GeV}$, $m_{\Lambda_b}=5.619 \ \text{GeV}$,
$m_{\Xi_c}=2.490 \ \text{GeV}$,
$m_{\Lambda}=1.116 \ \text{GeV}$ \cite{ParticleDataGroup:2022pth,Hu_2018}, and the light quarks $u$ and $d$ are taken as massless.  
On the other hand, the vacuum condensates are given by:  
$\left<\bar{q}q\right> = -(0.24 \pm 0.01\ \text{GeV})^3$, $\left<\bar{s}s\right> = (0.8 \pm 0.1) \left<\bar{q}q\right> $, $\left<g_s^2 GG \right> = 0.88 \pm 0.25\ \text{GeV}^4$, $\left< \bar{q} G q \right> = \left< \bar{q}g_s \sigma G q \right> = m_0^2 \ \left<\bar{q}q\right>$,  $\left< \bar{s} G s \right> = \left< \bar{s}g_s \sigma G s \right> = m_0^2\ \left<\bar{s}s\right>$ and $m_0^2= 0.8 \pm 0.1\ \text{GeV}^2$
at the energy scale $\mu = 1\ \text{GeV}$  \cite{Hu_2018,Xin:2023usd}. Finally, when setting the effective threshold at $\sqrt{s_0^{\Lambda_b}}=(6.5\pm 0.1)$ GeV, we find 
\begin{equation}
\lambda_{\Lambda_b}= 
\left( 3.4 \pm 0.2 \pm 0.6 \right) \times10^{-2} 
\ \left[\text{GeV}^3\right],
\end{equation}
where the first uncertainty originates from the uncertainties of the effective threshold $s_0^{\Lambda_b}$
and the Borel parameter $M^2$, the second one arises from the uncertainties of other
input parameters.
The dependence of the coupling constant $\lambda_{\Lambda_b}$ on the Borel parameter $M^2$ is illustrated in FIG.\ref{fig:coupling-constants} (a). 

% \begin{figure}
%     \centering
%     \includegraphics[width=0.52\textwidth]{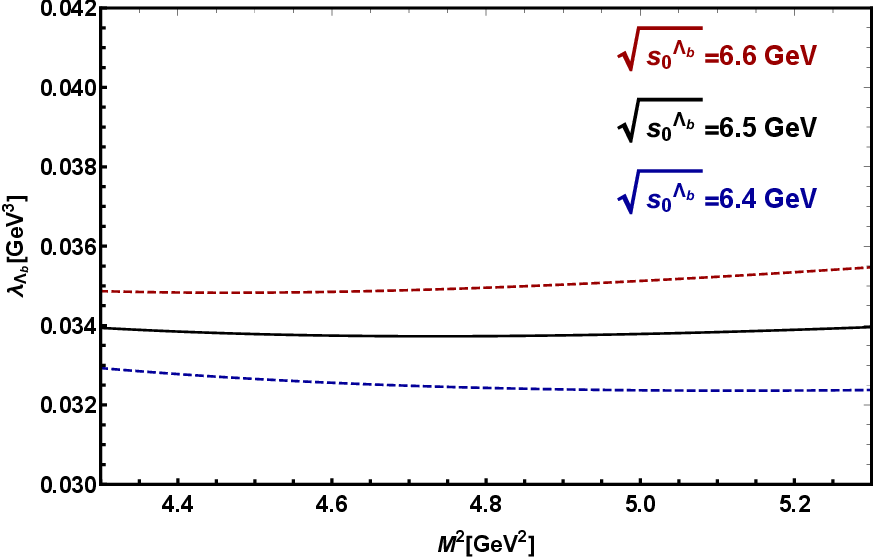}
%     \caption{The $M^2$-dependence of $\Lambda_b$ coupling constants in different effective threshold $s_0^{\Lambda_b}$.}
%     \label{fig:decay_constant_lambda_b}
% \end{figure}

\section{The coupling constant of $\Xi_Q$ baryon in QCD sum rules}{\label{Appen-QCD-input2}}

\begin{equation}{\label{eq:OPE_result2}}
                 \begin{aligned}
             % \mathcal{J}_{\Xi_Q} &= \epsilon^{ijk} \left[  d_i^T C \gamma_5 s_j \right] P_R Q_k, \\
        \mathbf{Im}\Pi^{(pert)}_{\Xi_Q, 0}(s) 
           &= \frac{m_Q^4}{2^{9}\pi^3} \left(   
           \frac{1}{x^2} - \frac{8}{x} +8x -  x^2
           -12ln(x)
           \right), \\
            \mathbf{Im} \Pi^{(\left< \bar{q}q \right>)}_{\Xi_Q, 0} (s) 
          &= 
          \frac{m_s\left[\left<\bar{s}s\right> -  2\left<\bar{q}q\right> \right]}{2^5\pi}  (1-x^2),
          \\
            \mathbf{Im} \Pi^{(\left< GG\right>)}_{\Xi_Q, 0} (s)
         &=  \frac{\left<g^2_s G^2\right>}{3 \cdot 2^{10} \pi^3} (1 + 4x-5x^2),
          \\
         \Pi^{(\left<\bar{q} G q \right>)}_{\Xi_Q, 0}(s) 
          &=  \frac{ m_s \left[6\left< \bar{q}Gq \right> + \left< \bar{s}Gs \right>\right]}{3 \cdot 2^6 \pi^2 (m_Q^2- s)} , \\
             \Pi^{(\left< \bar{q}q \right>^2)}_{\Xi_Q, 0} (s)
                 &=
                \frac{{\left< \bar{q}q \right>\left< \bar{s}s \right>}}{6(m_Q^2-s)},
                 \end{aligned} 
           \end{equation}
where $x= \frac{m_Q^2}{s}$. 
\begin{equation}
    \lambda_{\Xi_c} = \left( 2.9 \pm 0.2 \pm 0.3 \right) \times 10^{-2} \ \left[\text{GeV}^3 \right]
\end{equation}
The dependence of the coupling constant $\lambda_{\Lambda_b}$ on the Borel parameter $M^2$ is illustrated in FIG.\ref{fig:coupling-constants} (b). 
% \begin{figure}
%     \centering
%     \includegraphics[width=0.52\textwidth]{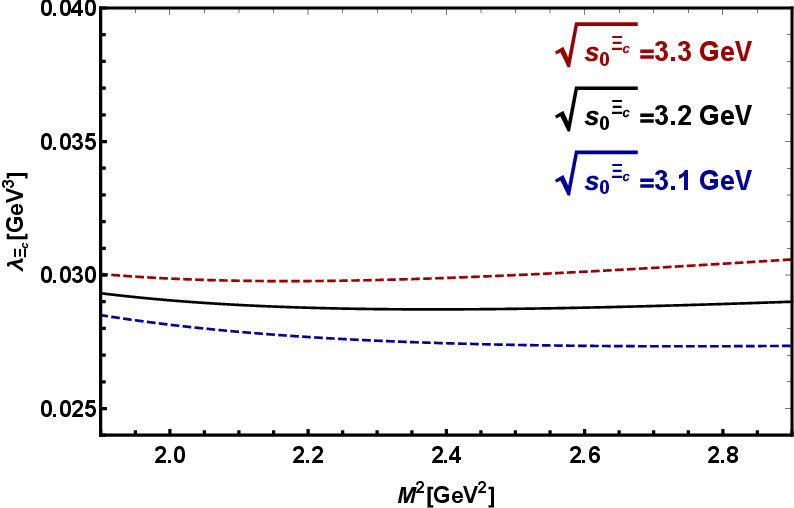}
%     \caption{The $M^2$-dependence of $\Xi_c$ coupling constants in different effective threshold $s_0^{\Xi_c}$.}
%     \label{fig:decay_constant_Xic}
% \end{figure}

\section{The coupling constant of $\Lambda$ baryon in QCD sum rules}{\label{Appen-Lambda}}

% \begin{figure}[!ht]
%     \centering
%     \includegraphics[width=0.52\textwidth]{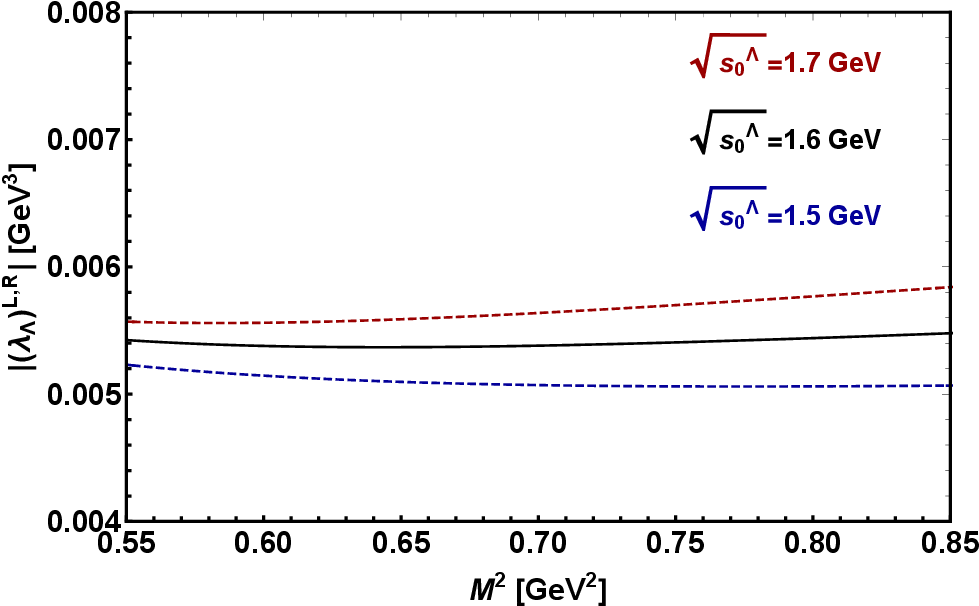}
%     \caption{The $M^2$-dependence of the coupling constants of $\Lambda$ in different threshold $\sqrt{s_0}$.}
%     \label{fig:decay_constant_lambda}
% \end{figure}

To evaluate the $\Lambda$ invisible decay in QCD sum rules, we have to estimate the corresponding coupling constants of $\Lambda$ baryon. 
When taking into account the leading order of $\alpha_s $ and the condensates up to dimension $d=6$, the OPE results are given by 
\begin{equation}{\label{eq:OPE_result_Lambda}}
                \begin{aligned}
    \mathbf{Im}\Pi_{\Lambda, 0}^{L, R (pert)}(s) 
    &= \frac{m_s^4}{2^{10}\pi^3} \left(   
           \frac{1}{x^2} - \frac{8}{x} +8x -  x^2
           -12ln(x)
           \right) ,
\\
    \mathbf{Im} \Pi^{L, R \left< \bar{q}q \right>}_{\Lambda, 0}(s) 
    &=   \frac{m_s \left<\bar{s} s\right> }{ 2^6 \pi}, 
\\
    \mathbf{Im} \Pi^{L,R \left< GG\right>}_{\Lambda, 0} (s)
        &=  \frac{\left<g^2_s G^2\right>}{3 \cdot 2^{11} \pi^3} (1 + 4x-5x^2),
\\
  \Pi^{L,R \left< \bar{q}G q \right>}_{\Lambda, 0}(s) 
  &=  \frac{ m_s  \left<\bar{s}Gs\right>}{3 \cdot 2^6 \pi^2 s},  \\
  % \Pi^{L/R(\left< \bar{q}q \right>^2)}_{\Lambda, 0}(s)
   %    &= 
   %    \frac{ m_s m_q \left<\bar{s}s \right> \left< \bar{q}\bar{q}\right>}{ 24  s^2}
                \end{aligned}
         \end{equation}
where $x= \frac{m_s^2}{s}$ and the mass of light quarks are neglected. When implementing the Borel transformation, the dependence of coupling constants on Borel parameters $M^2$ is illustrated in FIG.\ref{fig:coupling-constants} (c), which determine the value of coupling constants as
\begin{equation}
    |\lambda^{L,R}_{\Lambda}| = \left( 5.4 \pm 0.3\pm 0.1\right) \times 10^{-3}\ \left[\text{GeV}^3\right].
\end{equation}
With such coupling constants of $\Lambda$ baryon, the corresponding sensitivity on $|y_{\xi\phi}|$ are illustrated as the solid lines in FIG.\ref{fig:constraint-mchi} and FIG.\ref{fig:constraint-mtotal}.

\begin{figure}[htb]
    \centering
    \subfigure[]{
        \includegraphics[width=0.48\textwidth]{Fig/decay-constant-Lambda-b1.eps}}
    \subfigure[]{\includegraphics[width=0.48\textwidth]{Fig/decay-constant-Xic.eps}} \\
    \subfigure[]{\includegraphics[width=0.52\textwidth]{Fig/decay-constant-Lambda1.eps}}
    \caption{The $M^2$-dependence of $\Lambda_b \left(\Xi_c,  \Lambda \right)$ coupling constants in different effective threshold $s_0^{\Lambda_b \left(\Xi_c,  \Lambda \right)}$.}
    \label{fig:coupling-constants}
\end{figure}
